# Supplementary material for: Rumor Mitigation in Social Media Platforms with Deep Reinforcement Learning
Source: arXiv:2403.09217 source file (2024-03-14)
Supplement: Supplementary file 1 [file appendix.tex]

\section*{Appendix}
\appendix

\section{Baselines}\label{app::baseline}
We compare our model with the following methods.
\begin{itemize}[leftmargin=*]
    \item \textbf{Heuristic Search.}
    This method selects edges based on the topological characteristic such as degree (HSD)~\cite{holme2002attack,gao2011network} and betweenness centrality (HSC)~\cite{schneider2011suppressing,dey2017centrality}
    \item \textbf{Genetic Algorithm (GA)~\cite{bucur2016influence,parimi2021genetic}.}
    This method seeks better solution by updating the population iteratively.
    Through carefully designed operators, it generates new individuals and favor the fitter solution.
    \item \textbf{Simulated Annealing (SA)~\cite{li2017positive,biswas2021mcdm}.}
    This method is inspired by the physical annealing process and gradually decreases the temperature to explore better solutions in the solution space.
    \item \textbf{Pagerank (PR)~\cite{page1998pagerank}.}
    This method scores the importance of each node and removes the top K edges with the highest scores.
    \item \textbf{K-EDGEDELETION (KED)~\cite{tong2012gelling}.}
    Inspired by the edge-node mapping between original graph and the linear graph, this method quantifies the importance of edge by its' left and right eigen-scores independently.
    \item \textbf{Greedy with Bond Percolation (GBP)~\cite{kimura2008minimizing}.}
    This method selects the edge that minimizes the spread of rumor at each step using the Monte Carlo techniques~\cite{newman1999monte} based on the outcome of bond percolation method~\cite{kimura2007extracting}.
    \item \textbf{DRL Node Selection (DRLN)~\cite{meirom2021controlling}.}
    This recently proposed method introduces a RL framework for controlling partially-observed graph dynamics.
    It observes different stages of propagation and prioritizes candidates based on node embeddings calculated by GNNs.
\end{itemize}
